# Supplementary material for: DAMO: Deep Agile Mask Optimization for Full Chip Scale
Source: arXiv:2008.00806 source file (2020-11-16)
Supplement: Supplementary file 1 [file appendix.tex]

\section{Appendix}

\begin{table}[htb!]
  \caption{Architecture of DCGAN-HD}
  \centering
  
  \begin{tabular}{cccc}
      \toprule
      \multicolumn{4}{c}{High Resolution Generator for DCGAN-HD}                \\ 
      Layer               & Filter & Stride & Output Size    \\ \hline
      Input               & —      & —      & 1024$\times$1024$\times$3 \\
      Conv-BN-ReLU   & $7 \times 7$  & 1      & $1024  \times 1024  \times 32 $ \\
      Conv-BN-ReLU   & $3 \times 3$  & 2      & $512  \times 512  \times 64 $ \\
      Conv-BN-ReLU   & $3 \times 3$  & 2      & $256  \times 256  \times 128 $ \\
      Conv-BN-ReLU   & $3 \times 3$  & 2      & $128  \times 128  \times 256 . $ \\
      Conv-BN-ReLU   & $3 \times 3$  & 2      & $64   \times 64   \times 512$ \\
      Conv-BN-ReLU   & $3 \times 3$  & 2      & $32   \times 32   \times 1024$ \\
      Residual Block 1...9 & $3 \times 3$  & 1      & $32   \times 32   \times 1024$ \\
      Deconv-BN-ReLU & $3 \times 3$  & 2      & $64   \times 64   \times 512$ \\
      Deconv-BN-ReLU & $3 \times 3$  & 2      & $128  \times 128  \times 256$ \\
      Deconv-BN-ReLU & $3 \times 3$  & 2      & $256  \times 256  \times 128 $ \\
      Deconv-BN-ReLU & $3 \times 3$  & 2      & $512  \times 512  \times 64 $ \\
      Deconv-BN-ReLU & $7 \times 7$  & 1      & $1024 \times 1024 \times 3  $ \\ \hline
      \multicolumn{4}{c}{Discriminator $D_1$}                \\ \hline
      Input               & —            & — & $1024 \times 1024 \times 6$     \\
      Conv-BN-LeakyReLU      & $4 \times 4$ & 2 & $512 \times 512 \times 64$     \\
      Dropout (rate=0.5)  & —            & 1 & $512 \times 512 \times 64$     \\
      Conv-BN-LeakyReLU      & $4 \times 4$ & 1 & $512 \times 512 \times 128$     \\
      Dropout (rate=0.5)  & —            & 1 & $512 \times 512 \times 128$     \\
      Conv-BN-LeakyReLU      & $4 \times 4$ & 1 & $512 \times 512 \times 1$     \\ \hline
      \multicolumn{4}{c}{Discriminator $D_2$}                \\ \hline
      Input               & —            & — & $512 \times 512 \times 6$     \\
      Conv-BN-LeakyReLU      & $4 \times 4$ & 2 & $256 \times 256 \times 64$     \\
      Dropout (rate=0.5)  & —            & 1 & $256 \times 256 \times 64$     \\
      Conv-BN-LeakyReLU      & $4 \times 4$ & 1 & $256 \times 256 \times 128$     \\
      Dropout (rate=0.5)  & —            & 1 & $256 \times 256 \times 128$     \\
      Conv-BN-LeakyReLU      & $4 \times 4$ & 1 & $256 \times 256 \times 1$     \\ \bottomrule
    \end{tabular}
  \label{tab:DCGAN-HD}
\end{table}

\begin{algorithm}[h]
  \caption{Training algorithm of DAMO}
  \label{alg:maskopt}
  \small
  \begin{algorithmic}[1]
      \State Setting $\lambda_0$ $\lambda_1$ $\lambda_2$;
      \For {number of training iterations}
      \State Sample design patterns $\mathcal{W}\leftarrow \{w_1,\dots,w_b\}$;
      \State Sample mask patterns $\mathcal{X}\leftarrow \{x_1,\dots,x_b\}$;
      \State Sample wafer patterns $\mathcal{Y}\leftarrow \{y_1,\dots,y_b\}$;
      \State Initialize random noise $\mathcal{Z}_0\leftarrow \{{z_0}_1,\dots,{z_0}_b\}$;
      \State Initialize random noise $\mathcal{Z}\leftarrow \{{z}_1,\dots,{z}_b\}$;
      \State Concatenate $\mathcal{W}$, $\mathcal{Z}_0$ $\leftarrow \{\lbrace w_1, {z_0}_1 \rbrace,\dots,\lbrace w_b, {z_0}_b\rbrace \}$;
      \State $\Delta \vec{W}_{g} \gets {0}, \Delta \vec{W}_{d} \gets {0}$;
      \For {each $\lbrace  w_i, {z_0}_i\rbrace \in \mathcal{W}, \mathcal{Z}_0$, ${x}_i \in \mathcal{X}$, ${y}_i \in \mathcal{Y}$ and ${z}_i \in \mathcal{Z}$}
      \State $\hat{x}_i \gets G_{DMG}(w_i, {z_0}_i)$;
      % \State $E_0 = \lambda_0 \| \hat{y_0} - y\|_1$

      \State ${\mathcal{L}_g} \gets $ $-$ log$(D_{DMG}({w}_i, {\hat{{x}_i}}))+\lambda_0 \| {\phi({x}}_i)-\phi(\hat{ {{x}_i}})\|_1$;
      \State ${\mathcal{L}_d} \gets $ log$(D_{DMG}({{w}_i},{\hat{x}_i}))$ $-$ log$(D_{DMG}({{w}}_i, {{x}}_i))$

      \State Concatenate $\{\hat{x}_i, z_i\}$ for DLS input;
      \State Fix $\vec{W}_{g_{DLS}}$;
      \State ${{w}_r}_i \gets$ Remove SRAF in $w_i$ 
      \State $\hat{y}_i \gets G_{DLS}(\hat{{x}_i}, {z}_i)$;
      \State $\mathcal{L}_{g_{DLS}} \gets $ $-$ log$(D_{DLS}({x_i}, {\hat{y_i}}))+\lambda_1 \| \phi({y_i})-\phi(\hat{{y_i}})\|_1$;
      \State $\mathcal{L}_{d_{DLS}} \gets $ log$(D_{DLS}({x_i},{\hat{y}_i}))$ $-$ log$(D_{DLS}({x_i}, {y_i}))$
      % \State $E_1 = \lambda_1\| \hat{y}_i - y\|_1$
      \State $E = \lambda_2 \| \hat{y}_i - {{w}_r}_i\|_1$;
      % \State $\Delta \vec{W}_{g_{MO}} \gets \Delta \vec{W}_{g_{MO}} + $ $\frac{\partial E_0}{\partial \mathrm{\hat{y_0}_b}} \frac{\partial \mathrm{\hat{y_0}_b}}{\partial \vec{\mathrm{W}}_{g_0}}$ + $\frac{\partial E_2}{\partial \mathrm{\hat{y}_b}} \frac{\partial \mathrm{\hat{y}_b}}{\partial \vec{\mathrm{W}}_{g}}$ + $\frac{\partial E_2}{\partial \mathrm{\hat{y}_b}} \frac{\partial \mathrm{\hat{y}_b}}{\partial \vec{\mathrm{W}}_{g}}$
      \State ${\Delta \vec{W}_g} \gets {\Delta \vec{W}_g} + \dfrac{\partial {\mathcal{L}_g}}{\partial {\vec{W}_g}} + \dfrac{\partial \mathcal{L}_{g_{DLS}}}{\partial {\vec{W}_{g}}} + \dfrac{\partial E}{\partial {\vec{W}_g}}$; 
      \State ${\Delta \vec{W}_d} \gets {\Delta \vec{W}_d} + \dfrac{\partial {\mathcal{L}_d}}{\partial {\vec{W}_d}} + \dfrac{\partial \mathcal{L}_{d_{DLS}}}{\partial {\vec{W}_{d}}}$;
      % \State $\vec{W}_d \gets \vec{W}_d + \dfrac{\partial \mathcal{L}_d}{\partial \vec{W}_{d}}$;

      \EndFor
      \State $\vec{W}_{g} \gets \vec{W}_{g} - \dfrac{lr}{b}\Delta \vec{W}_{g}$;
      \State $\vec{W}_{d} \gets \vec{W}_{d} - \dfrac{lr}{b}\Delta \vec{W}_{d}$;
      % \State $\vec{W}_{d} \gets \vec{W}_{d} - \dfrac{lr}{b}\Delta \vec{W}_{d}$;
      \EndFor
  \end{algorithmic}
\end{algorithm}

$G_{DMG}$, $D_{DMG}$ and $G_{DLS}$ are parameterized as ${\vec{W}_g}$, ${\vec{W}_d}$ and ${\vec{W}_{g_{DLS}}}$ respectively.
Firstly, we sample a mini-batch of design/mask/wafer patterns as ground truth and initialize $\mathcal{Z}_0$/$\mathcal{Z}$ for mask and wafer prediction respectively (line 3--7).
Then, design $\mathcal{W}$ and $\mathcal{Z}_0$ are concatenated for mask generation (line 8).
Initially, the gradients of DMG are set to zeros (line 9).
DMG is trained and the outputs are pushed into DLS for wafer prediction (lines 10--19).
A $L_1$ loss $E$ is applied to narrow the difference between ground truth design $\vec{w_r}_i$ and predicted wafer pattern $\hat{y_i}$ (line 20).
In the training process, the parameters of $G_{DMG}$ are not only updated by $\dfrac{\partial {\mathcal{L}_g}}{\partial {\vec{W}_g}}$ but also guided by $\dfrac{\partial {\mathcal{L}_{g_{DLS}}}}{\partial {\vec{W}_g}}$ (line 21).
Similarly, $D_{DMG}$ is optimized by ${\mathcal{L}_d}$ and $\mathcal{L}_{d_{DLS}}$ (line 22).
Finally, the network gradients are calculated (lines 24--25).
